# Supplementary material for: SoK: Oracles from the Ground Truth to Market Manipulation
Source: arXiv:2106.00667 source file (2021-09-02)
Supplement: Supplementary file 1 [file 06-appendix.tex]

% !TEX root = ../main.tex

\appendix

%TODO need to align the images 

% \begin{figure}[b!]
%     \centering
%     \includegraphics[width=0.35\textwidth,height=0.9\textheight]{../graphs/data_flow_2_onchain_vertical.png}
%     \caption{Transaction workflow}
%     \label{fig:transaction_workflow}
% \end{figure}
